# Supplementary material for: Training Strategies for Isolated Sign Language Recognition
Source: arXiv:2412.11553 source file (2025-05-12)
Supplement: Supplementary file 1 [file appendix.tex]

\clearpage
\setcounter{page}{13}
\appendix

\onecolumn

\section*{Supplementary material}
\label{sec:supplementary}

\begin{figure*}[htp]
  \centering
  \includegraphics[width=0.8\linewidth]{images/dynamic_ges.jpg}
  \caption{The screenshots from the dynamic gesture recognition demo. The bounding boxes highlight detected gestures with their class labels. Each dynamic gesture is marked related to its function: yellow arrows indicate swipe directions, green and blue circles represent drag and drop, respectively, ``click" and ``double-click" display their corresponding gestures, green arrows or a stretchable blue rectangle for zoom gestures.}
  \label{fig: dynamic_ges}
\end{figure*}

\begin{figure*}[htp]
  \centering
  \includegraphics[width=0.93\linewidth]{images/gesture_tasks.png}
  \caption{Different tasks addressed by HaGRIDv2. (a) The gesture detector aims to predict a bounding box with a label for each hand on the image; (b) The gesture classifier produces a label for the entire image; (c) The hand detector recognizes all hands by bounding boxes with the same label ``hand"; (d) The gesture generator creates an image of a person showing a gesture according to the prompt.}
  \label{fig: tasks}
\end{figure*}

\begin{figure*}[htp]
  \centering
  \includegraphics[width=0.45\linewidth]{images/sbs_results.png}
  \caption{The SBS results compare Stable Diffusion 2.1 fine-tuned on the HaGRID and HaGRIDv2 datasets, as well as a comparison between HaGRIDv2 and the original Stable Diffusion 2.1 model.}
  \label{fig: sbs2}
\end{figure*}

\begin{figure*}[htp]
  \centering
  \includegraphics[width=0.6\linewidth]{images/no_gesture_samples.png}
  \caption{Samples of the ``no gesture" class in HaGRID and HaGRIDv2 datasets.}
  \label{fig: no_gesture_samples}
\end{figure*}

\begin{figure*}[htpb] % Измените htp на htpb
  \centering
  \includegraphics[width=0.8\linewidth]{images/auto_boxes.png}
  \caption{The pipeline for automatic image annotation. a) The higher hand on the one-handed gesture image is marked as the gesticulating hand; b) Two predicted boxes for the two-handed gesture are merged into a single box. c) A two-handed ``xsign" gesture is marked by a square bounding box, received by stretching a vertical line equal to the distance between two boxes.}
  \label{fig: auto}
\end{figure*}

\begin{table}
\begin{center}
\scalebox{0.6}{
\begin{tabular}{|p{1.0in}|p{2.3in}|p{1.0in}|p{2.3in}|}
\hline
Gesture & Applications & Gesture & Applications\\
\hline
thumb\_index & 
-- Input number 2 \newline
-- Mouse control on the screen \newline
-- Used for ZOOM and SWIPE dynamic gestures 
& point & 
-- Mouse control \newline
-- Activate smart home system by pointing \newline
-- Used for CLICK / DOUBLE CLICK / SWIPE dynamic gestures \\
\hline

thumb\_index2 & 
-- Screenshot of a specific area \newline
-- Start screen recording / sharing \newline
-- Take a selfie / screenshot \newline
-- Used for ZOOM dynamic gesture 
& pinkie & 
-- Input number 1 \newline
-- Set volume / brightness to minimum \\
\hline

middle\_finger & 
-- Express disapproval during a video conference \newline
-- Negative content rating 
& holy & 
-- Express a request during video conferences \newline
-- Switch to silent mode \newline
-- Play relaxing music or personal playlist \\
\hline

grip & 
-- Input number 0 \newline
-- Mute \newline
-- Give a negative (zero) rating \newline
-- Used for Drag-and-Drop dynamic gesture 
& grabbing & 
-- Move objects on the screen \newline
-- Used for Drag-and-Drop dynamic gesture \\
\hline

three3 & 
-- Input number 3 \newline
-- A humorous gesture to use during a video conference. It can be accompanied by a mask or stickers 
& timeout & 
-- Pause content \newline
-- Power off the system \newline
-- Emotional gesture during conversation (request to stop speaking). Mute the interlocutor / turn off the volume \\
\hline

take\_photo & 
-- Take a photo / screenshot / selfie \newline
-- Open a new window \newline
-- Start screen recording / sharing 
& xsign & 
-- Shut down the entire system \newline
-- Pause content \newline
-- Mute \newline
-- Report inappropriate content \\
\hline

three\_gun & 
-- Humorous gestures during video conferences, accompanied by stickers, fonts, or music \newline
-- Set the volume to maximum \newline
-- Turn on the music 
& heart & 
-- Express love during a video conference, accompanied by stickers, fonts, or music \newline
-- Like a song / video / add to playlist \\
\hline

\end{tabular}}
\end{center}
\caption{Gestures applications in gesture recognition systems. ``heart2" was not included as it has the same meaning as ``heart".}
\label{tabl:funcs}
\end{table}

\begin{figure*}[htp]
  \centering
  \includegraphics[width=0.8\linewidth]{images/hagrid_samples.jpg}
  \caption{Samples from HaGRIDv2 dataset.}
  \label{fig: hagrid_samples}
\end{figure*}

\begin{figure*}[htp]
  \centering
  \includegraphics[width=1.0\linewidth]{images/dyn_ges_scheme.jpg}
  \caption{The algorithm for recognizing dynamic gestures, exemplified by the ``zoom out" gesture.}
  \label{fig: dyn_ges_scheme}
\end{figure*}

\begin{table*}[htp]
\centering
\scalebox{0.7}{
\begin{tabular}{lccccc}
\hline
Model & Optimizer & Weight Decay & Learning Rate & Scheduler & Scheduler' Params.\\
\hline
ResNet & SGD & $1^{-4}$ & $1^{-1}$ & ReduceLROnPlateau & mode: min, factor: 0.1\\
MobileNetV3 & SGD & $5^{-4}$ & $5^{-3}$ & StepLR & step size: 30, gamma: 0.1\\
VitB16 & SGD & $5^{-4}$ & $5^{-3}$ & CosineAnnealingLR & T max: 8\\
ConvNext & AdamW & $5^{-2}$ & $4^{-3}$ & CosineAnnealingLR, LinearLR & T max: 8, factor: 0.001\\
SSDLite & SGD & $5^{-4}$ & $1^{-4}$ & StepLR & step size: 30, gamma: 0.1\\
YOLOv10 & SGD & $5^{-4}$ & $1^{-2}$ & LambdaLR & sinusoidal function\\
\hline
\end{tabular}}
\caption{Training hyperparameters.}
\label{tabl:params}
\end{table*}

\begin{figure*}[htp]
  \centering
  \includegraphics[width=0.8\linewidth]{images/samples.png}
  \caption{Samples from datasets, participated in cross-dataset evaluation and pre-trains impact experiment.}
  \label{fig: samples}
\end{figure*}

\begin{figure*}[htp]
  \centering
  \includegraphics[width=0.55\linewidth]{images/sbs.png}
  \caption{The interface for SBS evaluation presenting two images generated by two Stable Diffusion 2.1 models fine-tuned on HaGRID and HaGRIDv2 datasets. Crowdworkers are asked to assess these images based on two criteria: which hand posture appears more natural and which image better corresponds to the text query describing the gesture.}
  \label{fig: sbs}
\end{figure*}

\begin{figure*}[htp]
  \centering
  \includegraphics[width=0.65\linewidth]{images/gen_gest.jpg}
  \caption{Examples of generated images with three Stable Diffusion 2.1 models: original, fine-tuned on HaGRID, and fine-tuned on HaGRIDv2.}
  \label{fig: gen_gest}
\end{figure*}
